# Supplementary material for: ChipletQuake: On-die Digital Impedance Sensing for Chiplet and Interposer Verification
Source: arXiv:2504.19418 source file (2025-04-28)
Supplement: Supplementary file 1 [file 08-Appendices.tex]

% \section*{Appendices}

% \appendix
% \subsection*{A. Validation Tests For Bit Extractions} \label{ApxA}
